# Supplementary material for: GraphGPT: Graph Instruction Tuning for Large Language Models
Source: arXiv:2310.13023 source file (2024-05-07)
Supplement: Supplementary file 1 [file appendix.tex]

\appendix \section{Appendix}
\balance
\label{sec:appendix}

% In our provided appendix, we present the implementation details of text-graph grounding in Section~\ref{sec:tg_app}. Then, we summarize the statistical information of our datasets in Section~\ref{sec:ds}. Additionally, we present the further descriptions of baselines in Section~\ref{sec:baseline}. Additionally, utilized instruction templates for different tasks and datasets are presented in Section~\ref{sec:temp}. Finally, we provide supplementary experimental results in Section~\ref{sec:exp_sup}, including performance of link prediction and model case study. 

% In our provided appendix, we summarize the statistical information of our datasets in Section~\ref{sec:ds}. Then, we present the further descriptions of baselines in Section~\ref{sec:baseline}. Moreover, utilized instruction templates for different tasks and datasets are presented in Section~\ref{sec:temp}. Additionally, we present the implementation details of text-graph grounding in Section~\ref{sec:tg_app}. Finally, we provide supplementary experimental results in Section~\ref{sec:exp_sup}, including performance of link prediction and model case study. 

In the appendix, we provide a summary of the statistical information of our datasets in Section~\ref{sec:ds}. Furthermore, in Section~\ref{sec:baseline}, we offer detailed descriptions of the baseline methods used for comparison in our experiments. To facilitate the understanding of the instruction templates used for different tasks and datasets, we present them in Section~\ref{sec:temp}. These templates serve as guidelines for formulating instructions that are specific to the task and dataset at hand. In Section~\ref{sec:tg_app}, we present the implementation details of the text-graph grounding process. Finally, in Section~\ref{sec:exp_sup}, we provide supplementary experimental results.

\subsection{Statistical information of datasets}

\label{sec:ds}
The detailed statistical information of datasets is shown in Table~\ref{tab:ds}.
\begin{table}[h]
\centering
\vspace{-0.1in}
\caption{Statistical information of datasets.}\label{tab:ds}
\vspace{-0.1in}
\resizebox{.30\textwidth}{!}{\begin{tabular}{c|cccc} 
\hline
Dataset           & \# Nodes  & \# Edges  & \# Classes \\ 
\hline
ogb-arxiv         & 169,343   & 1,166,243 & 40         \\
PubMed            & 19,717    & 44,338    & 3          \\
Cora              & 25,120    & 182,280   & 70         \\
\hline
\end{tabular}}
\vspace{-0.1in}
\end{table}

\begin{table}[h]
\centering
\caption{Performance comparison of various instruction mixtures for link prediction on the PubMed dataset.}\label{tab:mix_2}
\vspace{-0.1in}
\resizebox{0.35\textwidth}{!}{\begin{tabular}{c|cc} 
\hline
Dataset                       & \multicolumn{2}{c}{PubMed}  \\ 
\hline
Model                         & AUC    & AP                 \\ 
\hline
MLP                           & 0.5583 & 0.5833             \\
GAT                           & 0.5606 & 0.6373             \\
GraphSAGE                          & 0.5041 & 0.5813             \\
RevGNN                        & 0.4538 & 0.5083             \\
Node2Vec                      & 0.6535 & 0.6885             \\ 
\hline
w/o Link                       & 0.5010 & 0.5005              \\
only Link                     & 0.6704  &  0.6087            \\
Arxiv-std + PubMed-std + Link & \textbf{0.8246} & \textbf{0.8026}             \\
Arxiv-mix + PubMed-mix + Link & 0.6451 & 0.5886             \\
\hline
\end{tabular}}
\vspace{-0.1in}
\end{table}
\begin{table}[h]
\centering
\caption{Instruction template for the graph matching task.}
    \label{tab:inst_temp_1}
    \vspace{-0.1in}
\small
\begin{tabularx}{0.5\textwidth}{X X}
    \toprule
     % \multicolumn{2}{c}{\textbf{Title}}  \\
     
     % \textbf{Input} & \textbf{Output} \\
     % Input: & Output: \\
     % \centering
      % \textbf{Graph Matching} \\
      \multicolumn{2}{@{}p{\linewidth}@{}}{\centering \textbf{Graph Matching}}  \\
      \midrule
      % \raggedright
      \textbf{Input:} Given a sequence of graph tokens \texttt{<graph>} that constitute a subgraph of a citation graph, where the first token represents the central node of the subgraph, and the remaining nodes represent the first and second order neighbors of the central node. Each graph token contains the title and abstract information of the paper at this node. Here is a list of paper titles: \texttt{\{1. Paper 1. 2. Paper 2. ... n. Paper n\}}, please reorder the list of papers according to the order of graph tokens (i.e., complete the matching of graph tokens and papers).\\
      \midrule
      \textbf{Output:} Based on the given graph tokens and the list of paper titles, we obtain the matching of graph tokens and papers as follows: \texttt{\{Graph token 1 corresponds to Paper Q, Graph token 2 corresponds to Paper P, ... Graph token n corresponds to Paper R\}}. \\

     \bottomrule
\end{tabularx}
\vspace{-0.1in}
\end{table}

\begin{table*}[h]
\vspace{-0.3in}
\centering
\caption{Instruction template for node classification and link prediction on different datasets.}
\vspace{-0.1in}
    \label{tab:inst_temp_2}
\small

\begin{tabularx}{1.02\textwidth}{X X}
    \toprule
     % \multicolumn{2}{c}{\textbf{Title}}  \\
     
     % \textbf{Input} & \textbf{Output} \\
     % Input: & Output: \\
      % \centering
      % \textbf{Node Classification (Arxiv in the COT manner)} \\
      \multicolumn{2}{@{}p{1.02\textwidth}@{}}{\centering \textbf{Node Classification (Arxiv in the COT manner)}} \\
      \midrule
      % \raggedright
      \textbf{Input:} Given a citation graph: \texttt{<graph>} where the 0th node is the target paper, with the following information: Abstract: \texttt{\{abstract of the central node\}}. Title: \texttt{\{title of the central node\}}. Question: Which arXiv CS sub-category does this paper belong to? Give 5 likely arXiv CS sub-categories as a comma-separated list ordered from most to least likely, in the form "cs.XX". Please think about the categorization in a step by step manner and avoid making false associations. Then provide your reasoning. \\
      \midrule
      \textbf{Output:} Based on the information, \texttt{\{reasoning process and answers\}}. \\
      \midrule
      % \centering
      % \textbf{Node Classification (Arxiv in the standard manner)} \\
      \multicolumn{2}{@{}p{1.02\textwidth}@{}}{\centering \textbf{Arxiv in the standard manner)}} \\
      \midrule
      % \raggedright
      \textbf{Input:} Given a citation graph: \texttt{<graph>} where the 0th node is the target paper, and other nodes are its one-hop or multi-hop neighbors, with the following information: Abstract: \texttt{\{abstract of the central node\}}. Title: \texttt{\{title of the central node\}}. Question: Which arXiv CS sub-category does this paper belong to? Give the most likely arXiv CS sub-categories of this paper directly, in the form "cs.XX" with full name of the category. \\
      \midrule
      \textbf{Output:} \texttt{\{the ground-truth answer\}}. \\
      \midrule
      % \centering
      % \textbf{Node Classification (PubMed in the COT manner)} \\
      \multicolumn{2}{@{}p{1.02\textwidth}@{}}{\centering \textbf{Node Classification (PubMed in the COT manner)}} \\
      \midrule
      % \raggedright
      \textbf{Input:} Given a citation graph: \texttt{<graph>} where the 0th node is the target paper, with the following information: Abstract: \texttt{\{abstract of the central node\}}. Title: \texttt{\{title of the central node\}}. Question: Does the paper involve any cases of Type 1 diabetes, Type 2 diabetes, or Experimentally induced diabetes? Please give one or more answers of either Type 1 diabetes, Type 2 diabetes, or Experimentally induced diabetes; if multiple options apply, provide a comma-separated list ordered from most to least related. Please think about the categorization in a step by step manner and avoid making false associations. Then provide your reasoning for each choice. \\
      \midrule
      \textbf{Output:} Based on the information, \texttt{\{reasoning process and answers\}}. \\
      \midrule
      % \centering
      % \textbf{Node Classification (PubMed in the standard manner)} \\
      \multicolumn{2}{@{}p{1.02\textwidth}@{}}{\centering \textbf{Node Classification (PubMed in the standard manner)}} \\
      \midrule
      % \raggedright
      \textbf{Input:} Given a citation graph: \texttt{<graph>} where the 0th node is the target paper, and other nodes are its one-hop or multi-hop neighbors, with the following information: Abstract: \texttt{\{abstract of the central node\}}. Title: \texttt{\{title of the central node\}}. Question: Which case of Type 1 diabetes, Type 2 diabetes, or Experimentally induced diabetes does this paper involve? Please give one answer of either Type 1 diabetes, Type 2 diabetes, or Experimentally induced diabetes directly. \\
      \midrule
      \textbf{Output:} \texttt{\{the ground-truth answer\}}. \\
      \midrule
      % \centering
      % \textbf{Node Classification (Cora in the COT manner)} \\
      \multicolumn{2}{@{}p{1.02\textwidth}@{}}{\centering \textbf{Node Classification (Cora in the COT manner)}} \\
      \midrule
      % \raggedright
      \textbf{Input:} Given a citation graph: \texttt{<graph>} where the 0th node is the target paper, with the following information: Abstract: \texttt{\{abstract of the central node\}}. Title: \texttt{\{title of the central node\}}. Question: Which of the following subcategories of computer science does this paper belong to: \texttt{\{1. Categories 1. 2. Categories 2. ... n. Categories n\}}? Give 5 likely categories as a comma-separated list ordered from most to least likely. Please think about the categorization in a step by step manner and avoid making false associations. Then provide your reasoning for each choice. \\
      \midrule
      \textbf{Output:} Based on the information, \texttt{\{reasoning process and answers\}}. \\
      \midrule
      % \centering
      % \textbf{Node Classification (Cora in the standard manner)} \\
      \multicolumn{2}{@{}p{1.02\textwidth}@{}}{\centering \textbf{Node Classification (Cora in the standard manner)}} \\
      \midrule
      % \raggedright
      \textbf{Input:} Given a citation graph: \texttt{<graph>} where the 0th node is the target paper, with the following information: Abstract: \texttt{\{abstract of the central node\}}. Title: \texttt{\{title of the central node\}}. Question: Which of the following subcategories of computer science does this paper belong to: \texttt{\{1. Categories 1. 2. Categories 2. ... n. Categories n\}}? Directly give the full name of the most likely category of this paper. \\
      \midrule
      \textbf{Output:} \texttt{\{the ground-truth answer\}}. \\
      \midrule
      % \centering
      % \textbf{Link Prediction (PubMed)} \\
      \multicolumn{2}{@{}p{1.02\textwidth}@{}}{\centering \textbf{Link Prediction (PubMed)}} \\
      \midrule 
      % \raggedright
      \textbf{Input:} Given a sequence of graph tokens: \texttt{<graph>} that constitute a subgraph of a citation graph, where the first token represents the central node of the subgraph, and the remaining nodes represent the first and second order neighbors of the central node. The information of the central node is as follow: Abstract: \texttt{\{abstract of the central node\}}. Title: \texttt{\{title of the central node\}}. The other sequence of graph tokens: \texttt{<graph>}, where the first token (the central node) with the following information: Abstract: \texttt{\{abstract of the central node\}}. Title: \texttt{\{title of the central node\}}. If the connections between nodes represent the citation relationships between papers, are these two central nodes connected? Give me a direct answer of "yes" or "no". \\
      \midrule
      \textbf{Output:} \texttt{\{the ground-truth answer\}}. \\

     \bottomrule
     
\end{tabularx}
\vspace{-0.1in}
\end{table*}

\vspace{-0.1in}
\subsection{Detailed Descriptions of Baselines}
\label{sec:baseline}
% For comprehensive performance comparison, our baseline set contains the following methods.
For a comprehensive performance comparison, our baseline set consists of the following methods which are presented below: \\\vspace{-0.12in}

\noindent\textbf{1) Conventional Deep Learning Methods}
\begin{itemize}[leftmargin=*]
\item \textbf{MLP}: This method employs a multilayer perceptron to independently encode different node representations.
\end{itemize}

\noindent\textbf{2) Graph Neural Encoders}
\begin{itemize}[leftmargin=*]
\item \textbf{GraphSAGE}~\cite{graphsage}: It is a framework designed for inductive representation learning on large graphs, enabling the efficient generation of node embeddings for previously unseen data. \\\vspace{-0.12in}
\item \textbf{GCN}~\cite{gcn}: This method extends the solution of convolutional neural networks to model graph-structured features. \\\vspace{-0.12in}
% \item \textbf{GAT}~\cite{gat}: It presents graph attention networks leveraging masked self-attentional layers to address the shortcomings of GCN. \\\vspace{-0.12in}
\item \textbf{GAT}~\cite{gat}: This method introduces graph attention networks that leverage masked self-attentional layers to address the limitations of GCN. It achieves this by differentiating the message passing among different nodes with weighted information aggregation. \\\vspace{-0.12in}
\item \textbf{RevGNN}~\cite{revgnn}: This work investigates several techniques, including reversible connections, group convolutions, weight tying, and equilibrium models, to enhance the memory and parameter efficiency of graph neural networks (GNNs). \\\vspace{-0.12in}
% \item \textbf{RevGNN}~\cite{revgnn}: This work explores reversible connections, group convolutions, weight tying, and equilibrium models to advance the memory and parameter efficiency of GNNs.
\end{itemize}

\noindent\textbf{3) Self-Supervised Graph Learning Approaches}
\begin{itemize}[leftmargin=*]
% \item \textbf{DGI}~\cite{DGI}: DGI maximizes mutual information between patch representations and corresponding high-level summaries of graphs to learn node representations within graph-structured data in an unsupervised manner.
\item \textbf{DGI}~\cite{DGI}: It maximizes the mutual information between patch representations and corresponding high-level summaries of graphs. By doing so, DGI enables the model to capture meaningful information from local patches of the graph and leverage it to learn informative node representations in an unsupervised manner.
\end{itemize}

\noindent\textbf{4) Graph Knowledge Distillation Frameworks}
\begin{itemize}[leftmargin=*]
\item \textbf{GKD}~\cite{GeoKD}: This method distills knowledge from a teacher GNN trained on a complete graph to a student GNN operating on a smaller or sparser graph. It achieves this by utilizing the Neural Heat Kernel (NHK) method, which encapsulates the geometric property of the underlying manifold. \\\vspace{-0.12in}
% \item \textbf{GLNN}~\cite{GLNN}: This work combines the benefits of GNNs and Multi-layer Perceptrons (MLPs) through knowledge distillation, eliminating inference graph dependency.
\item \textbf{GLNN}~\cite{GLNN}: This work combines the advantages of graph neural networks and MLPs using knowledge distillation, with the aim of removing the dependency on the inference graph.
\end{itemize}

\noindent\textbf{5) Graph Transformer Networks}
\begin{itemize}[leftmargin=*]
\item \textbf{NodeFormer}~\cite{NodeFormer}: This work leverages a kernelized Gumbel-Softmax operator to reduce the computational complexity of the graph transformer model, while also enabling the learning of latent graph structures from large graphs. \\\vspace{-0.12in}

\item \textbf{DIFFormer}~\cite{DIFFormer}: This work introduces an energy-constrained diffusion-based graph transformer. This transformer is designed to encode a batch of instances into evolutionary states by incorporating information from other instances. \\\vspace{-0.12in}
% It introduces an energy constrained diffusion-based graph transformer which encodes a batch of instances into evolutionary states that incorporate information from others. 
\end{itemize}

\noindent\textbf{6) Large Language Models}
\begin{itemize}[leftmargin=*]
\item \textbf{Baichuan-7B}~\cite{baichuan}: 
% Baichuan-7B is a bilingual (Chinese and English), open-source and large-scale pre-trained model with 7 billion parameters, based on the Transformer architecture, trained on approximately 1.2 trillion tokens.
It is an open-source, large-scale pre-trained model with 7 billion parameters. It is specifically designed to be bilingual, supporting both Chinese and English languages. This model has been trained extensively on a diverse range of data. \\\vspace{-0.16in}

\item \textbf{vicuna-7B-v1.1}~\cite{vicuna2023}: 
% It is an open-source chatbot that has been fine-tuned on user-shared conversations collected from ShareGPT using the Llama-1~\cite{llama} as the base model.
It is an open-source chatbot that has undergone fine-tuning using user-shared conversations collected from ShareGPT. The base model used for this fine-tuning is Llama-1, a reference to a specific model architecture. \\\vspace{-0.12in}

\item \textbf{vicuna-7B-v1.5}~\cite{vicuna2023}: This model is an enhanced iteration of vicuna-7b-v1.1, building upon Llama-2 as its base model.

\end{itemize}

\begin{table*}[h]
\vspace{-0.3in}
\centering
\caption{Comparison of our \model's predictions with ChatGPT on a arxiv paper (Continued).}
\vspace{-0.1in}
    \label{tab:case_2}
\small
\begin{tabularx}{1.02\textwidth}{X X}
    \toprule
     
    % \midrule
    \textbf{Title:} Greening Cloud-Enabled Big Data Storage Forensics: Syncany as a Case Study. (with \textbf{41} first-order and second-order neighbors) \\
      
      \midrule
      \textbf{Ground-Truth Category:} cs.CR, Cryptography and Security\\
      \midrule
      \textbf{ChatGPT (Node Content Only):} 
      Based on the title and abstract of the paper, we can make an educated guess about the likely arXiv CS sub-categories that this paper belongs to. Here is a step-by-step breakdown of the reasoning: 1. The paper mentions "cloud-enabled big data storage solutions" as the focus of investigation. This suggests that the paper is related to cloud computing and big data. 2. The paper also mentions "cyber forensics" and "investigation process" in the context of cloud-enabled big data platforms. This indicates that the paper is specifically about the forensic analysis of data stored in cloud-enabled big data platforms. Based on these observations, here are five likely arXiv CS sub-categories for this paper: 1. cs.DC (Distributed, Parallel, and Cluster Computing) - This sub-category covers topics related to distributed computing systems, which includes cloud computing. 2. cs.DB (Databases) - This sub-category covers topics related to database systems, which are often used in big data storage solutions. 3. cs.CR (Cryptography and Security) - This sub-category covers topics related to cyber security, which includes forensic analysis of digital evidence. 4. cs.SE (Software Engineering) - This sub-category covers topics related to software development and engineering, which may include the development of cloud-enabled big data storage solutions. 5. cs.CY (Computers and Society) - This sub-category covers topics related to the impact of computing on society, which may include the ethical and legal implications of forensic analysis in cloud-enabled big data storage. \\
      \midrule
      \textbf{ChatGPT (Node Content and Text-based Graph Structure):} 
      Based on the title of the paper "Greening Cloud Enabled Big Data Storage Forensics: Syncany as a Case Study" we can make an initial assumption that the paper belongs to the "Information Retrieval" (cs.IR) sub-category. However, to determine the most likely arXiv CS sub-categories, we need to analyze the content and context of the paper. 1. cs.DB (Databases): The paper focuses on cloud-enabled big data storage, which is closely related to databases. It discusses the identification, collection, analysis, preservation, and archiving of digital evidences in the context of Syncany private cloud storage service. This suggests that the paper may belong to the cs.DB sub-category. 2. cs.CR (Cryptography and Security): The paper addresses the forensic investigation of cloud-enabled big data storage platforms, which involves analyzing and recovering residual artifacts of criminal activities. This indicates a strong connection to the field of cybersecurity and digital forensics, which falls under the cs.CR sub-category. 3. cs.SE (Software Engineering): The paper may also belong to the cs.SE sub-category as it discusses the investigation process and the challenges involved in analyzing cloud-enabled big data storage platforms. It explores techniques and methodologies for locating and documenting residual artifacts of forensic value, which are relevant to the field of software engineering. 4. cs.CY (Computers and Society): The paper touches upon the societal impact of cloud-enabled big data storage and the need for efficient forensic investigation techniques. It highlights the potential reduction in time and resources spent on real-world investigations, which aligns with the concerns and issues addressed in the cs.CY sub-category. 5. cs.DC (Distributed, Parallel, and Cluster Computing): The paper mentions the decentralization of digital evidence acquisition in the context of BitTorrent Sync. This suggests a connection to distributed computing and parallel processing, which are topics covered in the cs.DC sub-category. Based on the above analysis, the likely arXiv CS sub-categories for the paper, ordered from most to least likely, are: cs.DB, cs.CR, cs.SE, cs.CY, cs.DC. \\
        \midrule
      \textbf{\model:} Based on the title and abstract of the paper, we can infer that the paper is related to cyber forensics and cloud-enabled big data storage. 
      \setlength\intextsep{0pt}
      \begin{wrapfigure}{l}{0.25\linewidth}
        \includegraphics[width=\linewidth]{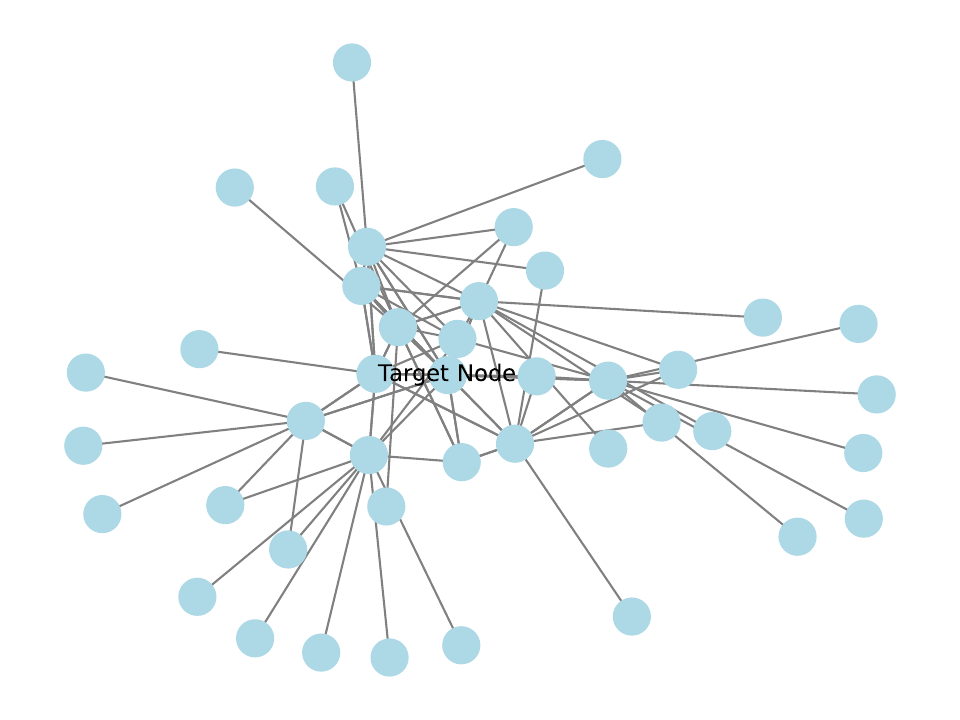}
    \end{wrapfigure}
      We can then proceed to categorize it based on the sub-categories of arXiv CS. 1. cs.CR: This category is for cryptography research, which involves the study of cryptographic algorithms, protocols, and systems. While the paper does not explicitly mention cryptography, it does involve the analysis of data remnants on a cloud-enabled big data platform, which could potentially involve cryptographic techniques. 2. cs.DS: This category is for database systems, which involves the design, implementation, and management of databases. The paper mentions the use of a popular storage engine for big data platforms, which suggests that the paper could be related to database systems. 3. cs.IR: This category is for information retrieval, which involves the study of how to effectively retrieve and organize information from large collections of data. The paper's focus on identifying and documenting residual artifacts of forensic value on a cloud-enabled big data platform suggests that it could be related to information retrieval. 4. cs.IT: This category is for information technology, which involves the study of the design, development, and use of information technology systems. The paper's focus on cloud-enabled big data storage and forensics suggests that it could be related to information technology. 5. cs.SY: This category is for systems and networking, which involves the study of computer systems and networks. The paper's focus on the analysis of data remnants on a cloud-enabled big data platform suggests that it could be related to systems and networking. \\

     \bottomrule
\end{tabularx}
\vspace{-0.1in}
\end{table*}

\vspace{-0.1in}
\subsection{Details of Text-Graph Grounding}
\label{sec:tg_app}
For the implementation details of Text-Graph Grounding~\ref{sec:TG_ground}, we follow previous work~\cite{G2P2}, aligning text features and graph features across three dimensions.
Mathematically, these dimensions can be represented by three sets of transformation equations:
\begin{align}
    g_1^{(1)}(\hat{\mathbf{H}}) = \{\hat{\mathbf{H}}_i, 1\leq i\leq N\}&, g_1^{(2)}(\hat{\mathbf{T}}) =  \{\hat{\mathbf{T}}_i, 1\leq i\leq N\} \nonumber \\
    g_2^{(1)}(\hat{\mathbf{H}}) = \{\hat{\mathbf{H}}_i, 1\leq i\leq N\}&, g_2^{(2)}(\hat{\mathbf{T}}) =  \{\frac{1}{|\mathcal{N}_i|}\sum_{j\in \mathcal{N}_i}\hat{\mathbf{T}}_j, 1\leq i\leq N\} \nonumber \\
    g_3^{(1)}(\hat{\mathbf{H}}) = \{\hat{\mathbf{T}}_i, 1\leq i\leq N\}&, g_3^{(2)}(\hat{\mathbf{T}}) =  \{\frac{1}{|\mathcal{N}_i|}\sum_{j\in \mathcal{N}_i}\hat{\mathbf{T}}_j, 1\leq i\leq N\}
\end{align}
where $\hat{\mathbf{H}}\in \mathbb{R}^{N\times d}$ denotes graph representations and $\hat{\mathbf{T}} \in \mathbb{R}^{N\times d}$ indicates text representations, and $N$ is the number of nodes.

% \subsection{Utilized Instruction Templates for Different Tasks and Datasets}
\vspace{-0.1in}
\subsection{Instruction Templates across Tasks/Data}
\label{sec:temp}

% To provide a more detailed demonstration of the instruction dataset we employed, we present the templates for different tasks (graph matching, node classification, and link prediction) on various datasets in the experiment, which is demonstrated in Table~\ref{tab:inst_temp_1} and~\ref{tab:inst_temp_2}.
% For all paper citation graphs, we adopt the same instruction template, whereas for specific downstream tasks, we design standard and COT (Chain-of-Thought) instruction templates for each dataset separately. Note that \texttt{<graph>} is the aforementioned indicator token and \texttt{\{...\}} denotes the blank that can be filled in.
% \vspace{-0.05in}
We provide instruction templates for different tasks (graph matching, node classification, and link prediction) on various datasets in our experiment. The templates are shown in Table~\ref{tab:inst_temp_1} and~\ref{tab:inst_temp_2}. While the same template is used for paper citation graphs, we design specific templates for each data in the downstream tasks, including both standard and COT (Chain-of-Thought) instructions. The \texttt{<graph>} token serves as an indicator, and \texttt{{...}} denotes fillable blanks.

\vspace{-0.1in}
\subsection{Supplementary Experimental Results}
\label{sec:exp_sup}
% In this subsection, we first delve into the performance of link prediction under different instruction mixtures. And then we compare the prediction results of our \model\ and ChatGPT under different instruction formats (\ie, with node content only, with node content and text-based graph structure, our designed graph instruction).
In this subsection, we analyze the link prediction performance using different instruction mixtures. We then compare the prediction results of our \model\ and ChatGPT under different instruction formats, including node content only, node content with text-based graph structure, and our custom-designed graph instruction.

% In the following subsection, we initiate our discourse by exploring the performance of link prediction, scrutinizing how it behaves under varying mixes of instructions. Our scrutiny is extended to a comparison of the predictive outcomes from ChatGPT and our specific model when they are subjected to different formats of instruction. These formats range from the provision of the node content solely, to the provision of the node content in conjunction with a text-based graph structure, and eventually to our uniquely designed graph instruction.

\vspace{-0.05in}
\subsubsection{\bf Performance of Link Prediction}
% We compared four different mixtures of instruction: i) COT instruction data for node classification only (w/o Link); ii) instruction data for link prediction only (only Link); iii) A mix of standard instruction data for node classification and instruction data for link prediction (Arxiv-std + PubMed-std + Link); iv) A mix of 50\% standard instruction data for node classification, 50\% COT instruction data for node classification, and instruction data for link prediction (Arxiv-mix + PubMed-mix + Link). When compared to representative baselines, as shown in Table~\ref{tab:mix_2}, the mixture of standard instruction data for node classification and instruction data for link prediction achieve results far exceeding the baseline. Moreover, according to the results of Table~\ref{tab:mix_1} mentioned earlier, this variant still outperforms SOTA approaches in node classification. We attribute this to the task of link prediction, which can further help our \model\ understand graph structural information, thereby promoting the tuning of node classification. The standard node classification instruction data does also not interfere with the model’s understanding of link prediction.
Four different instruction mixtures are compared:
i) COT instruction data for node classification only (w/o Link)
ii) Instruction data for link prediction only (only Link)
iii) A mix of standard instruction data for node classification and instruction data for link prediction (Arxiv-std + PubMed-std + Link)
iv) A mix of 50\% standard instruction for node classification, 50\% COT instruction data for node classification, and instruction for link prediction (Arxiv-mix + PubMed-mix + Link). When compared to representative baselines, as presented in Table~\ref{tab:mix_2}, the combination of standard instruction data for node classification and instruction for link prediction significantly outperformed the baselines. Furthermore, as mentioned earlier in Table~\ref{tab:mix_1}, this particular variant outperformed state-of-the-art approaches in node classification. This improvement can be attributed to the task of link prediction, which enhances our \model's understanding of graph structural information and facilitates node classification tuning. Importantly, the inclusion of node classification instructions does not impede the model's comprehension of link prediction.

\subsubsection{\bf Comparison Between ChatGPT and \model}
Table~\ref{tab:case_2} shows more comparison cases between ChatGPT and \model.
